# Supplementary material for: Magnetic Fluctuations, Precursor Phenomena and Phase Transition in MnSi under Magnetic Field
Source: arXiv:1606.07962 source file (2017-07-27)
Supplement: Supplementary file 1 [file PRL_Magnetic_field_Supplement_v13.pdf]

## DETERMINATION OF THE CORRELATION LENGTH

As a first step to deduce the correlation lengths $\xi$, the SANS patterns have been radial averaged to obtain $S(Q)$, i.e. the scattered intensity as a function of the momentum transfer $Q$. For the configurations where the magnetic field was along the neutron beam ($\vec{B}||\vec{k}_i$), $S(Q)$ is obtained by radial averaging the entire pattern. For the complementary direction where the field is perpendicular to the incident neutron beam ($\vec{B} \perp \vec{k}_i$), $S(Q)$ is obtained by radial averaging the intensity in two 30° wedges centered around $Q_Z = 0$, of which one is illustrated in Fig. **??**. Examples of the deduced $S(Q)$ for both field orientations for $B = 0.2$ T can be found in Fig. **??**(a)-(b). Next, $\xi$ is obtained by fitting $S(Q)$ to the Ornstein-Zernike function for fluctuating correlations convoluted with the instrumental resolution:

$$S(Q) = \frac{C}{(Q - 2\pi/\ell)^2 + 1/\xi^2}, \tag{1}$$

with $C$ the Curie constant and $\ell$ the pitch of the helix. The corresponding fits are indicated in Figs. **??**(a)-(b) as solid lines and the deduced temperature dependence of $\ell$ is displayed in Fig. **??**(c).

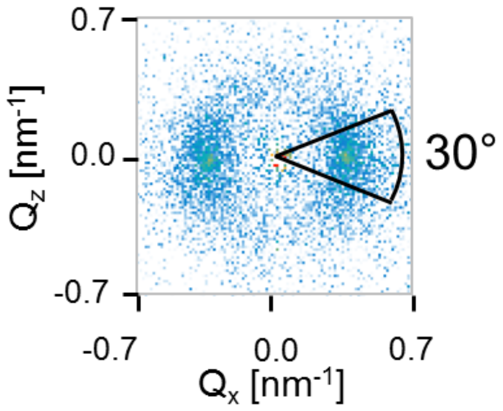


FIG. S1. This figure shows an example of a SANS pattern obtained in the configuration where the magnetic field is perpendicular to the neutron beam ($\vec{B} \perp \vec{k}_i$). The 30° wedge indicates the region for which $S(Q)$ is determined.

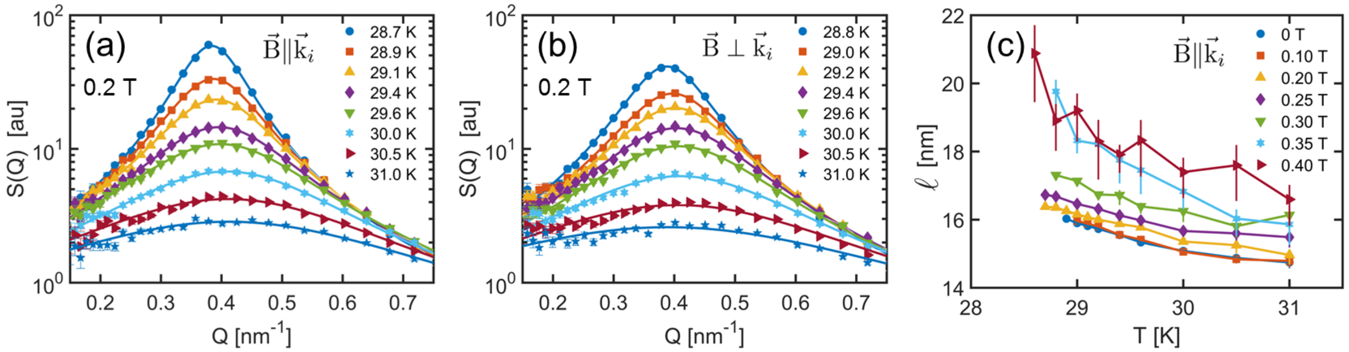


FIG. S2. SANS results obtained on LARMOR. Panel (a) and (b) show $S(Q)$ in arbitrary units at $B = 0.2$ T obtained for the configuration where $\vec{B}||\vec{k}_i$ and $\vec{B} \perp \vec{k}_i$, respectively. The solid lines indicate the best fits of eq. **??** convoluted with the instrumental resolution to $S(Q)$. Panel (c) displays the temperature dependence of the pitch of the helix $\ell$ for several magnetic fields applied along the neutron beam. $\ell$ is proportional to the ratio of the ferromagnetic exchange and the Dzyaloshinsky-Moriya (DM) constant.
